# Supplementary material for: FullPack: Full Vector Utilization for Sub-Byte Quantized Inference on General Purpose CPUs
Source: arXiv:2211.06982 source file (2022-11-20)
Supplement: Supplementary file 1 [file main.pdf]

---

# FULLPACK: FULL VECTOR UTILIZATION FOR SUB-BYTE QUANTIZED INFERENCE ON GENERAL PURPOSE CPUs

---

Anonymous Authors<sup>1</sup>

## A APPENDIX: ON-DEVICE MEASUREMENTS

executed instructions.

A complete demonstration of the results of our evaluation on fully connected layers of eleven different well-known CNN models are available in Figure 11.

## B APPENDIX: DETAILED EXECUTION METRIC ANALYSIS

Here, we provide more detailed information about the execution of each method. As depicted in Figure ??, *FullPack* outperforms the baseline, *Ruy-W8A8*. One may expect that with narrower bit-width, the speedup of *FullPack* to get better, but as discussed in § ?? and § ??, this is true only for *FullPack-W2A2* and not for *FullPack-W1A1*. As previously mentioned, the reason is that the instructions overhead becomes bottleneck in excution of *FullPack-W1A1*. For deeper inspection, we reported Instructions Count of each method for each model against the main baseline, *Ruy-W8A8* (Figure 12).

As we see, only when we quantize the activaitons, we still have  $0.73\times$  instructions compared to the baseline. The reason is that *Ruy-W8A8* needs more preprocessing to prepare the data for processing with respect to *FullPack*. However, *XNNPack-W8A8* needs way less instructions compared to both *FullPack* and *Ruy-W8A8*,  $0.68\times$  of *Ruy-W8A8*.

This, however, does not explain the reason behind why *FullPack* is faster than *XNNPack-W8A8* for models with larger sizes. To investigate more, we evaluated Instructions Per Cycle (IPC) for each method. Figure 13 reports our results. Here, *FullPack* has better IPC than the baseline for almost all models and all sizes. However, if we compare the IPC of *XNNPack-W8A8* with *FullPack* we can observe that *FullPack* has better IPC than the *XNNPack-W8A8* for larger sizes of all the models, except *W8A4*, which causes *FullPack* to be faster than *XNNPack-W8A8*, even with more

---

<sup>1</sup>Anonymous Institution, Anonymous City, Anonymous Region, Anonymous Country. Correspondence to: Anonymous Author <anon.email@domain.com>.

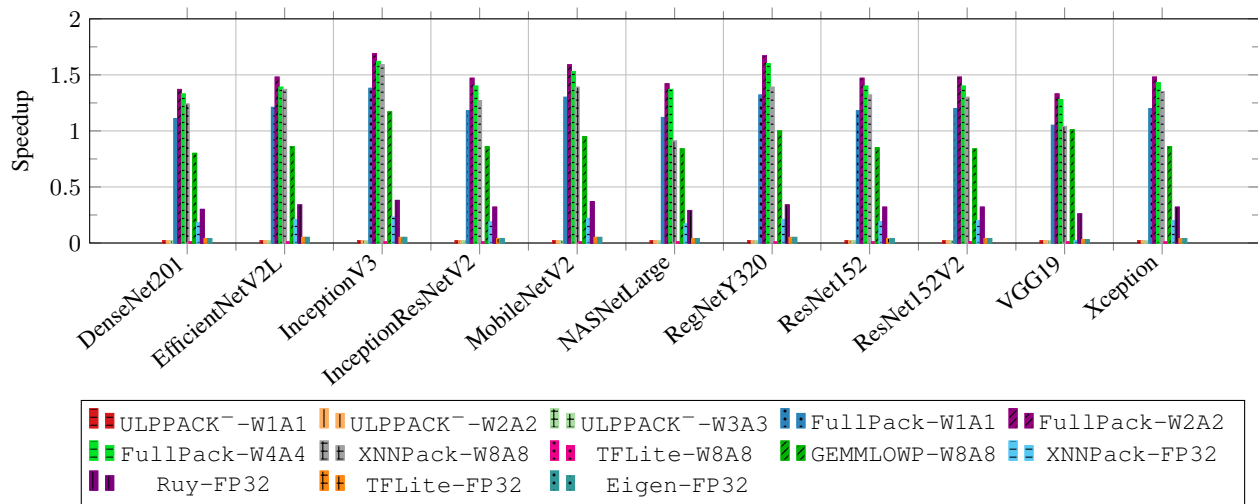

Figure 11. Speedup of each method against Ruy-W8A8 on Fully Connected layers of a few well-known Convolutional Neural Networks on Raspberry Pi 4 Model B.

## Appendix - FullPack: Full Vector Utilization for Sub-Byte Quantized Inference on General Purpose CPUs

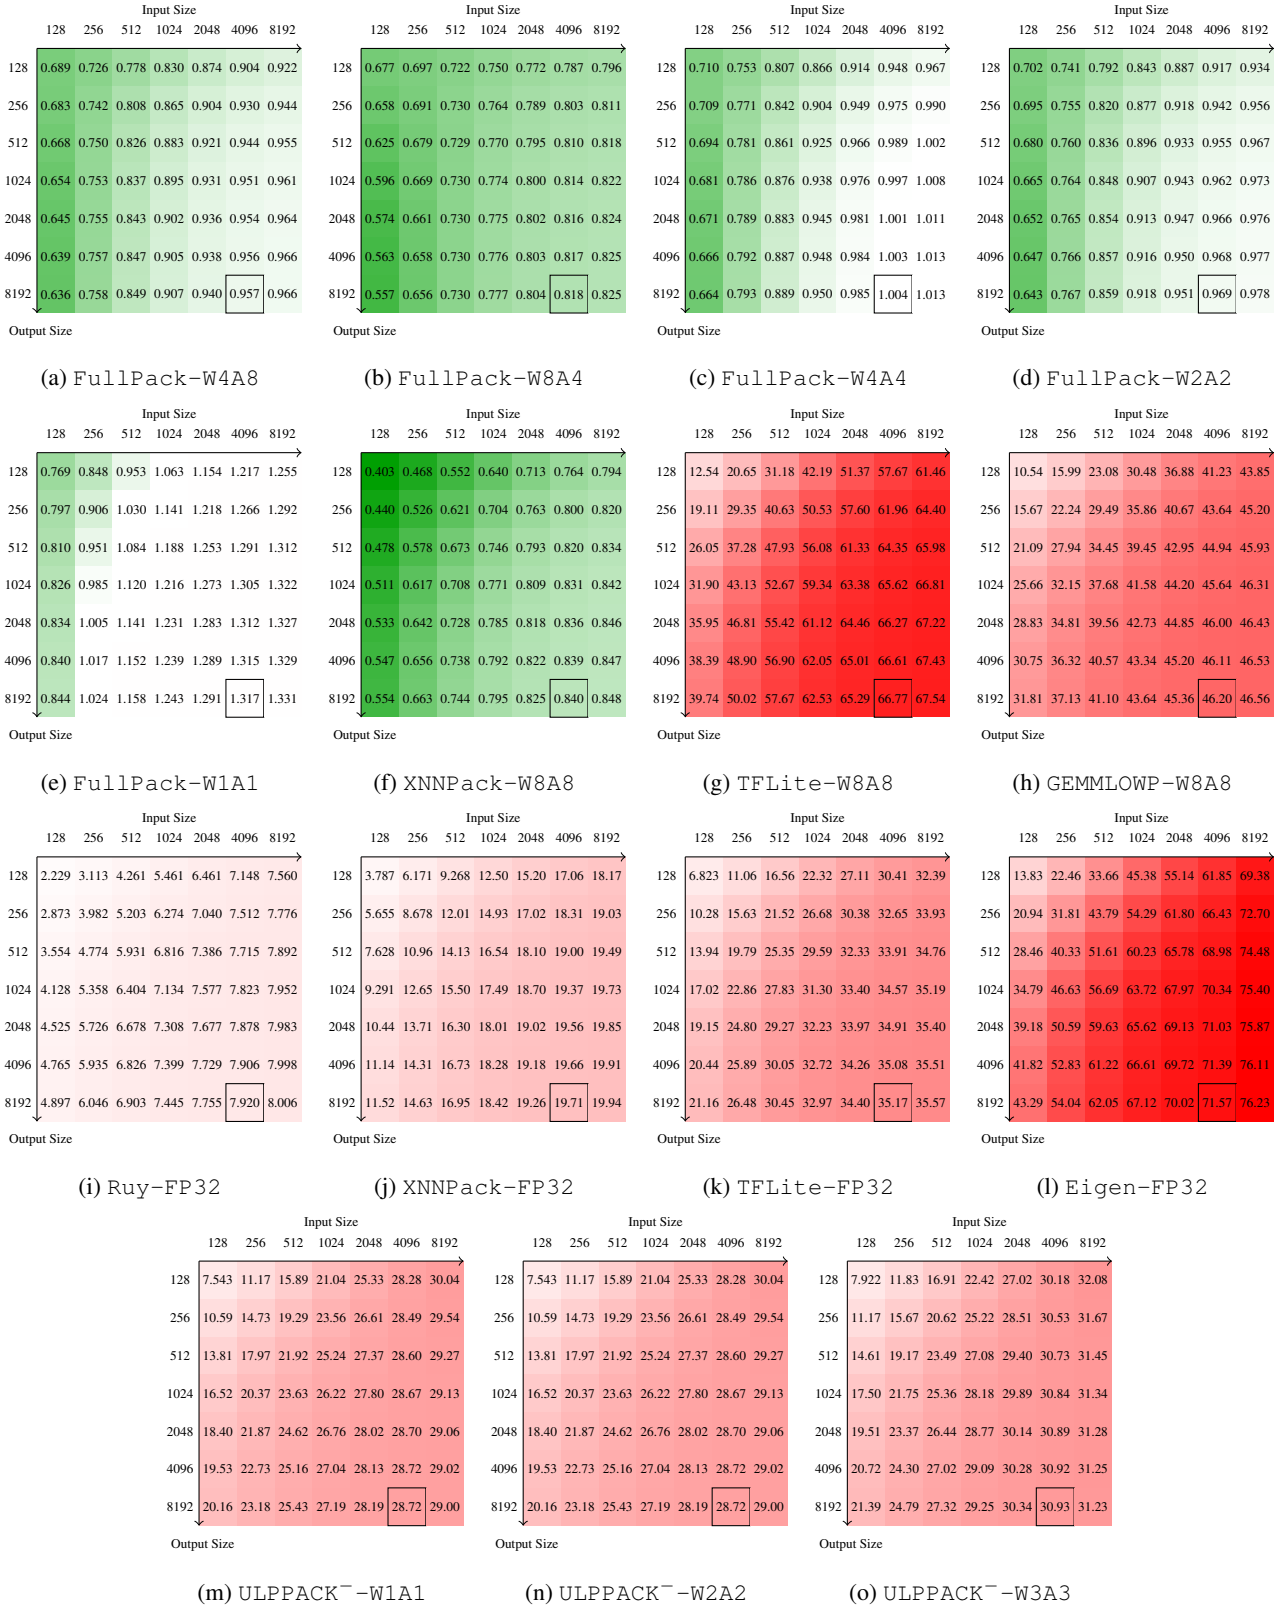

Figure 12. Instruction Count comparison (Increase;  $I_{case}/I_{baseline}$ ) of different methods on various IO sizes of a FullyConnected layer against the baseline (Ruy-W8A8). The number of cells reports the increase multiplier.

## Appendix - FullPack: Full Vector Utilization for Sub-Byte Quantized Inference on General Purpose CPUs

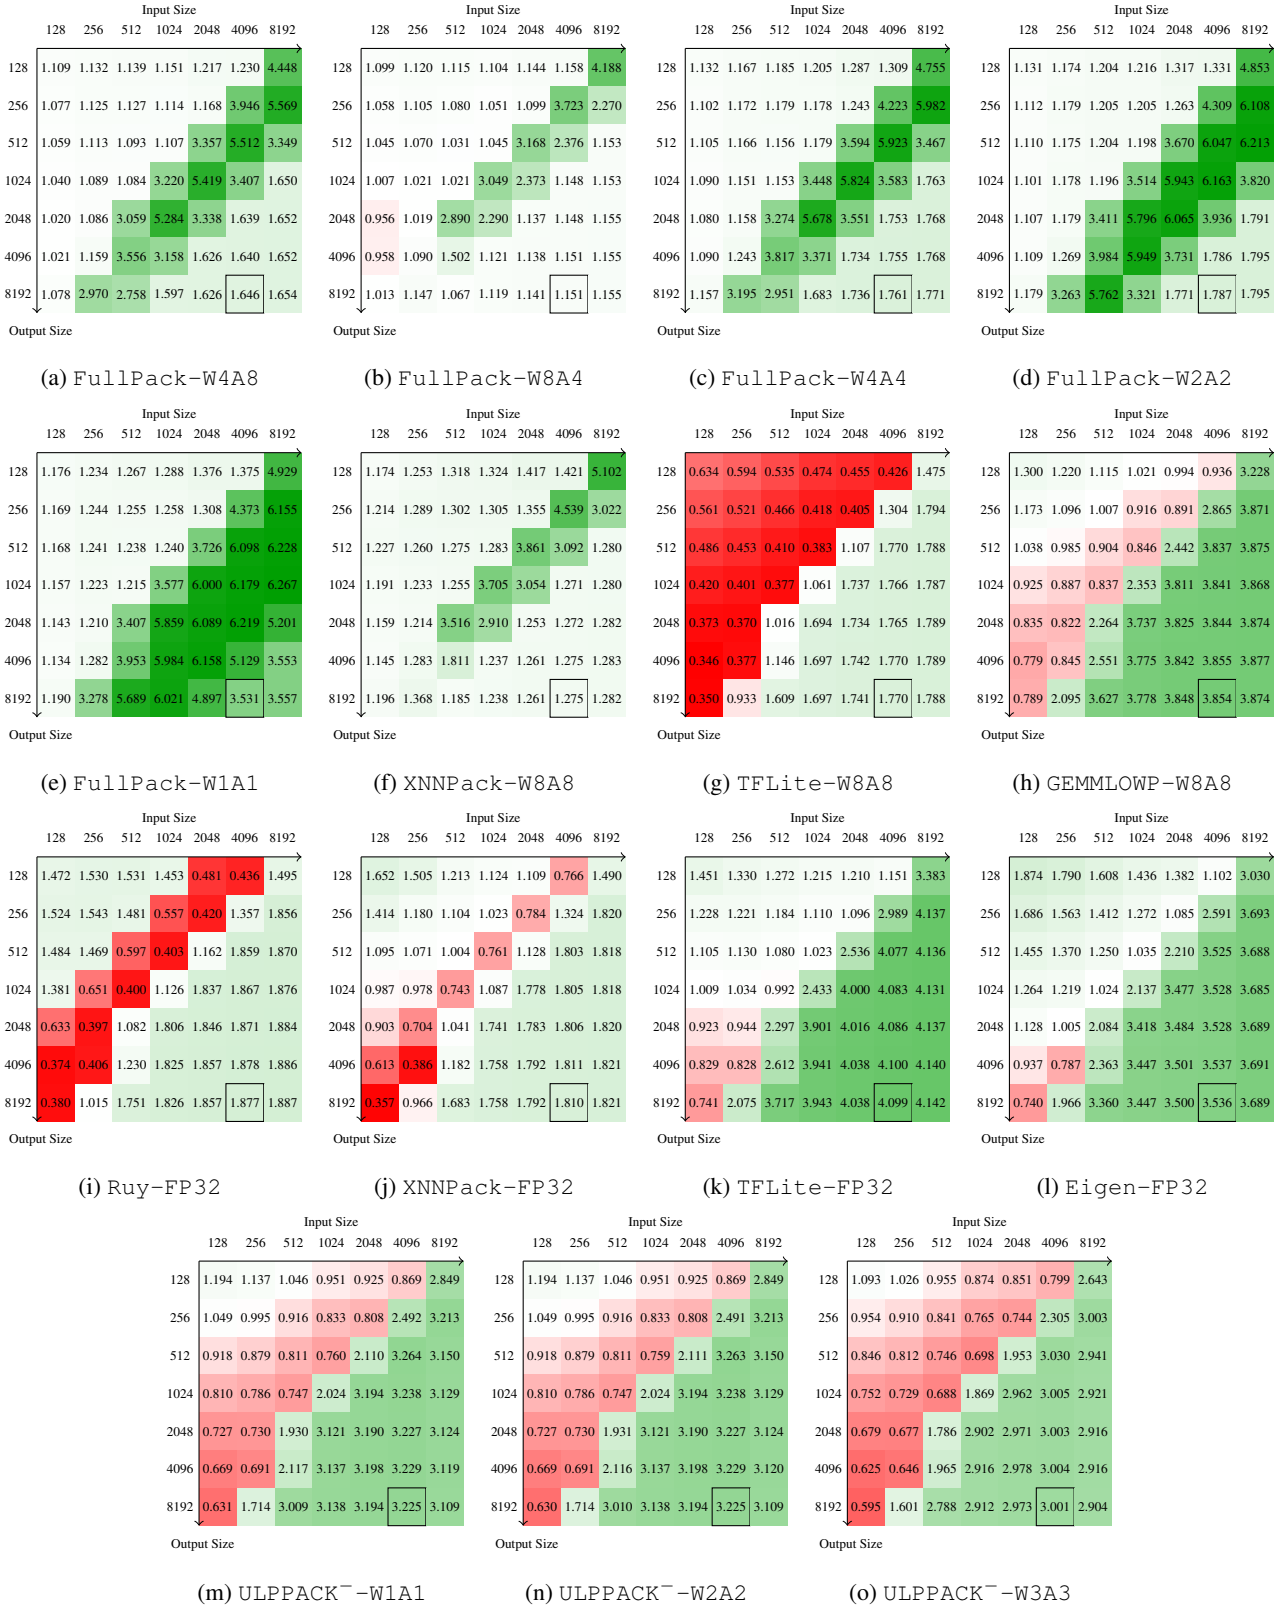

Figure 13. IPC (Instruction Per Cycle) comparison (Increase;  $IPC_{case}/IPC_{baseline}$ ) of different methods on various IO sizes of a FullyConnected layer against the baseline (Ruy-W8A8). The number of cells reports the increase multiplier.
